# Supplementary material for: Catastrophe by Design in Population Games: Destabilizing Wasteful Locked-in Technologies
Source: arXiv:2007.12877 source file (2020-07-25)
Supplement: Supplementary file 1 [file appendix.tex]

\section{Appendix 2}\label{app:appendix_2}

\subsection*{Appendix A}

\begin{definition}
    Given parameters $T \ge 0$ and $\gamma \in (0, 1)$ we define
    \begin{equation*}
        \bar f(x; T, \gamma) = 2x - (1 + \gamma) - T\ln\frac{x}{1 - x},~x \in (0, 1)
    \end{equation*}
\end{definition}

\begin{lemma}\label{lem:PrFeBnd}
    Given a function $f(x; T, \gamma) = \bar f(x; T, \gamma) + \epsilon(x)$ with domain $\dom f = (0, 1)$ and parameters $T \ge 0$ and $\gamma \in (0, 1)$ such as $|\epsilon(x)| \le \epsilon$ for some $\epsilon \in (0, \min\{\gamma, 1 - \gamma\})$ and $\forall x \in (0, 1)$ it holds
    \begin{equation*}
        \bar f(x; T, \gamma + \epsilon) \le f(x; T, \gamma) \le \bar f(x; T, \gamma - \epsilon)
    \end{equation*}
\end{lemma}
\begin{proof}
    
    By assumption $\forall \gamma \in (0, 1)$
    \begin{equation*}
        \epsilon \in (0, \min\{\gamma, 1 - \gamma\})
        \implies \epsilon \in (0, \gamma)
        \implies \gamma - \epsilon \in (0, \gamma) \subseteq (0, 1)
    \end{equation*}
    And, similarly, $\gamma + \epsilon \in (\gamma, 1) \subseteq (0, 1)$
    
    Then, by definition, $\forall x \in (0, 1)$
    \begin{equation*}\begin{aligned}
        |\epsilon(x)| \le \epsilon
        \implies& |f(x; T, \gamma) - \bar f(x; T, \gamma)| \le \epsilon\\
        \implies& \bar f(x; T, \gamma) - \epsilon\le f(x; T, \gamma) \le \bar f(x; T, \gamma) + \epsilon\\
        \implies& 2x - (1 + \gamma) - T\ln\frac{x}{1 - x} - \epsilon \le f(x; T, \gamma) \le 2x - (1 + \gamma) - T\ln\frac{x}{1 - x} + \epsilon\\
        \implies& 2x - (1 + (\gamma + \epsilon)) - T\ln\frac{x}{1 - x} \le f(x; T, \gamma) \le 2x - (1 + (\gamma - \epsilon)) - T\ln\frac{x}{1 - x}\\
        \implies& \bar f(x; T, \gamma + \epsilon) \le f(x; T, \gamma) \le \bar f(x; T, \gamma - \epsilon)
    \end{aligned}\end{equation*}
    
\end{proof}

\stef{
\begin{lemma}
$f\(x;T,\gamma\)$ is decreasing in $\gamma$.
\end{lemma}
\begin{proof}
\[\frac{\partial}{\partial \gamma} f\(x;T,\gamma\)=-1<0\]
Hence \[\bar f\(x;T,\gamma-\epsilon\)<\bar f\(x;T,\gamma\)+\epsilon\(x\)=f\(x;T,\gamma\)<f\(x;T,\gamma+\epsilon\)\]
\end{proof}
}

\begin{definition}
    Given $T \in [0, \frac{1}{2}]$ and $\gamma \in (0, 1)$, we define $x^*(T; \gamma) = min\{x: \bar f(x; T, \gamma) = 0\}$
\end{definition}

\begin{definition}
    Given $T \in [0, \frac{1}{2}]$, we define $x_1(T) = \frac{1 - \sqrt{1 - 2T}}{2}$ and $x_2(T) = \frac{1 + \sqrt{1 - 2T}}{2}$
\end{definition}

\begin{definition}
    Given $\gamma \in (0, 1)$, we define $T_c(\gamma)$ to be the unique $T$ such as $\bar f(x_2(T), T; \gamma) = 0$
\end{definition}

\begin{lemma}\label{lem:PrTcBnd}
    $\forall \gamma \in (0, 1)$ it holds
    \begin{equation*}
        0 < T_c(\gamma) < \frac{1}{2}
    \end{equation*}
\end{lemma}
\begin{proof}

    Let $g(T) = \sqrt{1 - 2T} - T\ln\frac{1 + \sqrt{1 - 2T}}{1 - \sqrt{1 - 2T}}$ with $\dom g = (0, \frac{1}{2})$.
    Then, by definition, $\forall \gamma \in (0, 1)$
    \begin{equation*}\begin{aligned}
        \bar f(x_2(T_c(\gamma)), T_c(\gamma); \gamma) = 0
        \implies& \sqrt{1 - 2T_c(\gamma)} - \gamma - T_c(\gamma)\ln\frac{1 + \sqrt{1 - 2T_c(\gamma)}}{1 - \sqrt{1 - 2T_c(\gamma)}} = 0\\
        \implies& g(T_c(\gamma)) = \gamma
    \end{aligned}\end{equation*}
    Hence, since $\dom g \subseteq (0, \frac{1}{2})$ it follows $0< T_c(\gamma) < \frac{1}{2},~\forall \gamma \in (0, 1)$.
    
\end{proof}

\begin{lemma}\label{lem:PrTcDec}
    $T_c(\gamma)$ is monotonically decreasing in $(0, 1)$
\end{lemma}
\begin{proof}
    
    By definition, $\forall \gamma \in (0, 1)$
    \begin{equation*}
        \bar f(x_2(T_c(\gamma)), T_c(\gamma); \gamma) = 0
        \implies \sqrt{1 - 2T_c(\gamma)} - \gamma - T_c(\gamma)\ln\frac{1 + \sqrt{1 - 2T_c(\gamma)}}{1 - \sqrt{1 - 2T_c(\gamma)}} = 0
    \end{equation*}
    
    Using implicit differentiation and Lemma~\ref{lem:PrTcBnd}
    \begin{equation*}\begin{aligned}
        &\frac{d}{d\gamma}f(x_2(T_c(\gamma)), T_c(\gamma); \gamma) = 0\\
        \implies& - \frac{T_c(\gamma)T_c'(\gamma)}{\sqrt{1 - 2T_c(\gamma)}} - 1 - T_c'(\gamma)\ln\frac{1 + \sqrt{1 - 2T_c(\gamma)}}{1 - \sqrt{1 - 2T_c(\gamma)}} + \frac{T_c(\gamma)T_c'(\gamma)}{\sqrt{1 - 2T_c(\gamma)}} = 0\\
        \implies& T_c'(\gamma) = - \frac{1}{\ln\frac{1 + \sqrt{1 - 2T_c(\gamma)}}{1 - \sqrt{1 - 2T_c(\gamma)}}} < 0
    \end{aligned}\end{equation*}
    Hence, $T_c(\gamma)$ is monotonically decreasing in $(0, 1)$
    
\end{proof}

\begin{proposition}
    Given a function $f(x; T, \gamma) = \bar f(x; T, \gamma) + \epsilon(x)$ with domain $\dom f = (0, 1)$ and parameters $\gamma \in (0, 1)$ and $T \ge 0$ such as $|\epsilon(x)| \le \epsilon$ for some $\epsilon \in (0, \min\{\gamma, 1 - \gamma\})$, then $\forall T > T_c(\gamma - \epsilon)$ it holds
    \begin{equation}
        f(x; T, \gamma) < 0,~\forall x \in (x^*(T;\gamma - \epsilon), 1) \supset [\frac{1}{2}, 1)
    \end{equation}
\end{proposition}
\begin{proof}
    
    Let $T > T_c(\gamma - \epsilon)$.
    Then, following our main analysis, it holds $\bar f(x; T, \gamma - \epsilon) < 0,~ \forall x \in (x^*(T, \gamma - \epsilon), 1) \supset [\frac{1}{2}, 1)$ and, our claim follows by Lemma~\ref{lem:PrFeBnd}.
    
\end{proof}

\begin{proposition}
    Given a function $f(x; T, \gamma) = \bar f(x; T, \gamma) + \epsilon(x)$ with domain $\dom f = (0, 1)$ and parameters $\gamma \in (0, 1)$ and $T \ge 0$ such as $|\epsilon(x)| \le \epsilon$ for some $\epsilon \in (0, \min\{\gamma, 1 - \gamma\})$, then $\forall T < T_c(\gamma - \epsilon)$ it holds
    \begin{equation*}
        f(x; T, \gamma) < 0,~\forall x \in (x^*(T;\gamma - \epsilon), \frac{1}{2})
    \end{equation*}
\end{proposition}
\begin{proof}
    
    Let $T \le T_c(\gamma - \epsilon)$.
    Then, following our main analysis, it holds $\bar f(x; T, \gamma - \epsilon) < 0,~ \forall x \in (x^*(T, \gamma - \epsilon), \frac{1}{2})$ and, our claim follows by Lemma~\ref{lem:PrFeBnd}.
    
\end{proof}

\begin{proposition}
    Given a function $f(x; T, \gamma) = \bar f(x; T, \gamma) + \epsilon(x)$ with domain $\dom f = (0, 1)$ and parameters $\gamma \in (0, 1)$ and $T \ge 0$ such as $|\epsilon(x)| \le \epsilon$ for some $\epsilon \in (0, \min\{\gamma, 1 - \gamma\})$, then it holds
    \begin{equation*}
        f(x; T, \gamma) > 0,~\forall x \in (0, x^*(T;\gamma + \epsilon))
    \end{equation*}
\end{proposition}
\begin{proof}
    
    Let $T \ge 0 $.
    Then, following our main analysis, it holds $\bar f(x; T, \gamma + \epsilon) > 0,~ \forall x \in (0, x^*(T, \gamma + \epsilon))$ and, our claim follows by Lemma~\ref{lem:PrFeBnd}.
    
\end{proof}

\begin{lemma}\label{lem:PrFPrimeBnd}
    Given $\gamma \in (0, 1)$ and $T \in [0, \infty)$ , then $\forall x \in (0, 1)$
    \begin{equation*}
        2 \le \bar f'(x; T, \gamma) \le 2 - 4T
    \end{equation*}
\end{lemma}
\begin{proof}
    
    Let $x \in (0, 1)$.
    Then
    \begin{equation*}\begin{aligned}
        \bar f''(x; T, \gamma) \le 0
        \implies& \frac{T(1 - 2x)}{x^2(1 - x)^2} \le 0\\
        \implies& 1 - 2x \le 0\\
        \implies& x \ge \frac{1}{2}
    \end{aligned}\end{equation*}
    
    Hence, $\forall x \in (0, 1)$ it follows that $\bar f'(x; T, \gamma) \le \bar f'(\frac{1}{2}) = 2 - 4T$
    
    Furthermore, $\lim_{t \to 0^+}\bar f'(t; T, \gamma) = \lim_{t \to 1^-}\bar f'(t; T, \gamma) = 2$, which, by continuity implies that $\bar f'(t; T, \gamma) \in (2, 2 - 4T),~\forall x \in (0, 1)$
    
\end{proof}

\begin{theorem}
    Given $\gamma \in (0, 1)$ and $T \in (0, \infty)$, then $\forall \epsilon \in (0, \min\{\gamma, 1 - \gamma\})$
    \begin{equation*}
        |x^*(T;\gamma - \epsilon) - x^*(T;\gamma + \epsilon)| \le \min\{\frac{\epsilon}{|1 - 2T|}, \frac{1}{2}\}
    \end{equation*}
\end{theorem}
\begin{proof}
       Using Taylor's Approximation on $x^*(T;\gamma - \epsilon)$, it follows that $\forall x \in (0, 1)$ there exists some $\lambda(x) \in [\min\{x^*(T;\gamma - \epsilon), x\}, \max\{x^*(T;\gamma - \epsilon), x\}]$ such that
    \begin{equation*}\begin{aligned}
        &\bar f(x; T, \gamma - \epsilon) = \bar f(x^*(T;\gamma - \epsilon); T, \gamma - \epsilon) + \bar f'(\lambda(x); T, \gamma - \epsilon)(x - x^*(T;\gamma - \epsilon))\\
        \implies& f(x; T, \gamma) + \epsilon = \bar f'(\lambda(x); T, \gamma - \epsilon)(x - x^*(T;\gamma - \epsilon))\\
        \implies& \bar f(x; T, \gamma + \epsilon)= \bar f'(\lambda(x); T, \gamma - \epsilon)(x - x^*(T;\gamma - \epsilon)) - 2\epsilon
    \end{aligned}\end{equation*}
    
    Hence, for $x = x^*(T;\gamma + \epsilon)$ and by Lemma \ref{lem:PrFPrimeBnd} we have
    \begin{equation*}\begin{aligned}
        &\bar f(x^*(T;\gamma + \epsilon); T, \gamma + \epsilon)= \bar f'(\lambda(x^*(T;\gamma + \epsilon)); T, \gamma - \epsilon)(x^*(T;\gamma + \epsilon) - x^*(T;\gamma - \epsilon)) - 2\epsilon\\
        \implies& x^*(T;\gamma + \epsilon) - x^*(T;\gamma - \epsilon) = \frac{2\epsilon}{\bar f'(\lambda(x^*(T;\gamma - \epsilon)); T, \gamma - \epsilon)}\\
        \implies& |x^*(T;\gamma + \epsilon) - x^*(T;\gamma - \epsilon)| = \frac{2\epsilon}{|\bar f'(\lambda(x^*(T;\gamma - \epsilon)); T, \gamma - \epsilon)|}\\
        \implies& |x^*(T;\gamma + \epsilon) - x^*(T;\gamma - \epsilon)| \le \frac{\epsilon}{|1 - 2T|}
    \end{aligned}\end{equation*}
    
    Finally, since $x^*(T;\gamma) \in (0, \frac{1}{2}),~\forall \gamma \in (0,1)$, our claim follows.   
\end{proof}
\subsection*{Appendix B}

\begin{lemma}\label{lem:PrMonG}
    $f(x) = \left(1 - \frac{1}{x}\right)^{x - 1}$ is monotonically decreasing in $(1, \infty)$
\end{lemma}
\begin{proof}

    Since $f(x)$ is differentiable in $(1, \infty)$, $f$ is monotonically decreasing in $(1, \infty)$ if a and only if $\forall x \ge 1$, $f'(x) < 0$.

    Let $g(x) = \ln\left(1 - \frac{1}{x}\right) + \frac{1}{x}$
    \begin{equation*}\begin{aligned}
        g'(x) > 0
        \iff& \frac{1}{1- \frac{1}{x}}\frac{1}{x^2} - \frac{1}{x^2} > 0\\
        \iff& \frac{1}{x^2(x - 1)} > 0\\
        \iff& x > 1
    \end{aligned}\end{equation*}
    Hence, $\forall x > 1$
    \begin{equation*}
        g(x)
        < \lim_{t \to \infty}g(t)
        = \lim_{x \to \infty}\left(\ln\left(1 - \frac{1}{x}\right) + \frac{1}{x}\right)
        = 0
    \end{equation*}
    
    And, thus, $\forall x > 1$
    \begin{equation*}\begin{aligned}
        f'(x)
        &= \left(\ln\left(1 - \frac{1}{x}\right) + \frac{x - 1}{1 - \frac{1}{x}}\frac{1}{x^2}\right)\left(1 - \frac{1}{x}\right)^{x - 1}\\
        &= \left(\ln\left(1 - \frac{1}{x}\right) + \frac{1}{x}\right)\left(1 - \frac{1}{x}\right)^{x - 1}\\
        &= g(x)\left(1 - \frac{1}{x}\right)^{x - 1}\\
        &< 0
    \end{aligned}\end{equation*}
    
\end{proof}

\begin{corollary}\label{cor:PrGAxisBnd}
    $\forall x \ge 2$
    \begin{equation*}
        \left(1 - \frac{1}{x}\right)^{x - 1} \le \frac{1}{2}
    \end{equation*}
    with equality only if $x = 2$
\end{corollary}
\begin{proof}

    Let $f(x) = \left(1 - \frac{1}{x}\right)^{x - 1}$.
    Then, by Lemma \ref{lem:PrMonG}, it follows that $f(x)$ is monotonically decreasing in $[2, \infty)$.
    Hence, $\forall x \ge 2$
    \begin{equation*}
        f(x) \le f(2) = \frac{1}{2}
    \end{equation*}
    with equality only if x = 2
    
\end{proof}

\begin{lemma}\label{lem:PrGBnd}
    $\forall \alpha \ge 2$ and $\forall p \in (0, 1)$
    \begin{equation*}
        p^{\alpha - 1}(1 - p) - \frac{1}{2\alpha} \le 0
    \end{equation*}
    with equality only if $\alpha = 2$ and $p = \frac{1}{2}$
\end{lemma}
\begin{proof}

    Let $f(\alpha, p) = p^{\alpha - 1}(1 - p) - \frac{1}{2\alpha}$.
    Then $\forall \alpha \ge 2$ and $\forall p \in (0, 1)$
    \begin{equation*}\begin{aligned}
        \frac{\partial}{\partial \alpha}f(\alpha, p) \le 0
        \iff& (\alpha - 1)p^{\alpha - 2}(1 - p) - p^{\alpha - 1} \le 0\\
        \iff& p^{\alpha - 2}((\alpha - 1)(1 - p) - p) \le 0\\
        \iff& (\alpha - 1)(1 - p) - p \le 0\\
        \iff& p \ge \frac{\alpha - 1}{\alpha}
    \end{aligned}\end{equation*}
    with equality only if $p =  \frac{\alpha - 1}{\alpha}$
    
    Hence, by Corollary \ref{cor:PrGAxisBnd}, $\forall \alpha \ge 2$ and $\forall p \in (0, 1)$
    \begin{equation*}\begin{aligned}
        f(\alpha, p)
        &\le f(\alpha, \frac{\alpha - 1}{\alpha})\\
        &= \left(\frac{\alpha - 1}{\alpha}\right)^{\alpha - 1}\left(1 - \frac{\alpha - 1}{\alpha}\right)-\frac{1}{2\alpha}\\
        &= \frac{1}{\alpha}\left(\left(1 - \frac{1}{\alpha}\right)^{\alpha - 1}-\frac{1}{2}\right)\\
        &\le 0
    \end{aligned}\end{equation*}
    with equality only if $\alpha = 2$ and $p = \frac{a - 1}{a} = \frac{1}{2}$

\end{proof}

\begin{lemma}\label{lem:PrMonF}
    $\forall \alpha \ge 2$ and $\forall p \in (0, 1)$
    \begin{equation*}
        p^\alpha(1 - p) + p(1 - p)^\alpha \le \frac{1}{2\alpha}
    \end{equation*}
    with equality only if $\alpha = 2$ and $p = \frac{1}{2}$
\end{lemma}
\begin{proof}

    Let $f(\alpha, p) = p^{\alpha - 1}(1 - p) - \frac{1}{2\alpha}$.
    Then, by Lemma \ref{lem:PrGBnd}, $\forall \alpha \ge 2$ and $\forall p \in (0, 1)$
    \begin{equation*}\begin{aligned}
       p^\alpha(1 - p) + p(1 - p)^\alpha - \frac{1}{2\alpha}
       &= p\left(p^{\alpha - 1}(1 - p) - \frac{1}{2\alpha}\right) + (1 - p)\left((1 - p)^{\alpha - 1}p - \frac{1}{2\alpha}\right)\\
       &= pf(\alpha, p) + (1 - p)f(\alpha, 1 - p) \le 0
    \end{aligned}\end{equation*}
    with equality only if $\alpha = 2$ and $p = 1 - p = \frac{1}{2}$
    
\end{proof}

\begin{lemma}\label{lem:PrExRootF}
    Given a function $f(x) = x^{\alpha - 1} - (1 - x)^{\alpha - 1} - \gamma - T\ln\frac{x}{1 - x}$ with domain $\dom f = (0, 1)$ and parameters $\alpha \ge 3$, $\gamma \in (0, 1)$, and $T \ge 0$ there exists a $x_0 \in (0, \frac{1}{2})$ such as $f(x_0) = 0$
\end{lemma}
\begin{proof}

    $\forall \alpha \ge 3$, $\forall \gamma \in (0, 1)$, $\forall T \ge \frac{1}{2}$, it holds:
    \begin{enumerate}[label=\alph*)]
        \item $\lim_{t \to 0^+}f(t) = \lim_{t \to 0^+}\left(t^{\alpha - 1} - (1 - t)^{\alpha - 1} - \gamma - T\ln\frac{t}{1 - t}\right) = \infty$, and
        \item $f(\frac{1}{2}) = - \gamma < 0$
    \end{enumerate}
    
    Hence, since $f$ is continuous in $(0, 1)$, by Bolzano's theorem that there exists $x_0 \in (0, \frac{1}{2})$ such as $f(x_0)$.
    
\end{proof}

\begin{theorem}
    Given a function $f(x) = x^{\alpha - 1} - (1 - x)^{\alpha - 1} - \gamma - T\ln\frac{x}{1 - x}$ with domain $\dom f = (0, 1)$ and parameters $\alpha \ge 3$, $\gamma \in (0, 1)$, and $T \ge \frac{1}{2}$, there exists a unique $x_0 \in (0, \frac{1}{2})$ such as:
    \begin{enumerate}[label=\arabic*)]
        \item $f(x_0) = 0$,
        \item $f(x) > 0,~\forall x \in (0, x_0)$, and
        \item $f(x) < 0,~\forall x \in (x_0, 1)$
    \end{enumerate}
\end{theorem}
\begin{proof}

    By Lemma \ref{lem:PrMonF}, $\forall \alpha \ge 3$, $\forall \gamma \in (0, 1)$, $\forall T \ge \frac{1}{2}$ and $\forall x \in (0, 1)$
    \begin{equation*}\begin{aligned}
        f'(x)
        &= (\alpha - 1)x^{\alpha - 2} + (\alpha - 1)(1 - x)^{\alpha - 2} - \frac{T}{x(1 - x)}\\
        &= \frac{a - 1}{x(1 - x)}\left(x^{\alpha - 1}(1 - x) + x(1 - x)^{\alpha - 1} - \frac{T}{\alpha - 1}\right)\\
        &\le \frac{a - 1}{x(1 - x)}\left(x^{\alpha - 1}(1 - x) + x(1 - x)^{\alpha - 1} - \frac{1}{2(\alpha - 1)}\right)\\
        &\le 0
    \end{aligned}\end{equation*}
    with equality only if $T = \frac{1}{2}$, $\alpha = 3$ ($\alpha - 1 = 2$), and $x = \frac{1}{2}$
    
    Hence, $f$ is decreasing in $(0, 1)$, and monotonic in $(0, \frac{1}{2})$ and $(\frac{1}{2}, 1)$.
    
    By Lemma \ref{lem:PrExRootF} there exists $x_0 \in (0, \frac{1}{2})$ such as $f(x_0) = 0$ and the claim follows by the following observations:
    \begin{enumerate}[label=\roman*)]
        \item Since, $f$ is monotonically decreasing in $(\frac{1}{2}, 1)$ it follows $f(x) \le f(\frac{1}{2}) < 0,~\forall x \in (\frac{1}{2}, 1)$, and
        \item Since, $f$ is monotonically decreasing in $(0, \frac{1}{2})$, it follows $f(x) < f(x_0) = 0,~\forall x \in (0, x_0)$, and $f(x) > f(x_0) = 0,~\forall x \in (x_0, \frac{1}{2})$.
    \end{enumerate}
    
\end{proof}

\begin{lemma}\label{lem:PrMinF}
    $\forall \alpha > 1$ and $x \in (0, 1)$
    \begin{equation*}
        x^\alpha + (1 - x)^\alpha \ge \frac{1}{2^{\alpha - 1}}
    \end{equation*}
\end{lemma}
\begin{proof}
    Let $f(X) = x^\alpha + (1 - x)^\alpha$. 
    Then $\forall x \in (0, 1)$
    \begin{equation*}\begin{aligned}
        f'(x) = 0
        \iff& \alpha\left(x^{\alpha - 1} - (1 - x)^{\alpha - 1}\right) = 0\\
        \iff& x = 1 - x\\
        \iff& x = \frac{1}{2}
    \end{aligned}\end{equation*}
    
    Furthermore $f''(x) = \alpha(\alpha - 1)\left(x^{\alpha - 1} + (1 - x)^{\alpha - 1}\right) > 0,~\forall \alpha > 1$.
    Hence, $\forall x \in (0, 1)$ and $\forall \alpha > 1$
    \begin{equation*}
        f(x) \ge f(\frac{1}{2}) = \frac{1}{2^{\alpha - 1}}
    \end{equation*}
    with equality only if $x = \frac{1}{2}$
    
\end{proof}
